# Supplementary material for: ManiVideo: Generating Hand-Object Manipulation Video with Dexterous and Generalizable Grasping
Source: arXiv:2412.16212 source file (2024-12-18)
Supplement: Supplementary file 1 [file 12_appendix.tex]

% \section{Experiment Setting}

\textcolor{red}{Please refer to the demo video for more dynamic results.} 

\section{Our Dataset}
\label{sec:appendix_section}

\begin{figure}
    \centering
    \includegraphics[width=1.\linewidth]{fig_imgs/data.png}
    \caption{A sampling of our data.}
    \label{fig:data}
\end{figure}
We train our ManiVideo on three types of datasets.
For object data, we utilize Objaverse~\cite{deitke2023objaverse}, and human data is sourced from Human4DiT~\cite{shao2024human4dit}.
For HOI video data, in addition to the public DexYCB dataset~\cite{chao2021dexycb}, We collect third-person view videos of participants standing and interacting with objects using bimanual hands.
Specifically, our dataset contains 722 videos (376k frames) depicting daily tool-use behaviors covering 15 objects, 10 views and 8 participants.
Compared to other datasets~\cite{liu2024taco, fan2023arctic}, our data is human-centric and free from distractions caused by irrelevant objects (e.g., tables), making it particularly suitable for downstream applications like human-based HOI video generation in~Sec.\ref{sub:app}.
As illustrated in Fig.~\ref{fig:data}, the dataset comprises human-centered videos captured from multiple views using both long-focus and short-focus cameras.

\noindent{\textbf{Object model acquisition.}}
We utilize the 3D object models from TACO~\cite{liu2024taco} as our objects, with meshes consisting of up to 100K triangular faces to capture fine-grained geometric details. Specifically, we select commonly used objects from daily life, including spoons, shovels, bowls, cups, and boxes.

\noindent{\textbf{Data Capturing.}}
Similar to TACO~\cite{liu2024taco}, hand motion is extracted from multi-view RGB videos, whereas object motion is captured using a motion capture system by tracking four markers affixed to the object's surface.
Moreover, our data capture system combines 12 synchronized industrial FLIR cameras with a NOKOV optical motion capture setup equipped with six Mars4H infrared cameras.

\noindent{\textbf{Data Annotating.}}
We process hands and objects as separate entities. 
For hands, we employ RTMpose~\cite{jiang2023rtmpose} to differentiate between the left and right hands and extract 2D keypoints. 
Subsequently, the MANO model is utilized to represent the 3D hand mesh, which is optimized using both 2D and 3D loss functions. 
For a detailed description of the process, please refer to TACO~\cite{liu2024taco}.

For objects, the 6D pose, comprising rotation and translation, is obtained using the motion capture system. 
Marker-to-surface correspondence is then optimized, and the refined object poses are computed by integrating the relative positions of markers on the object mesh with the captured marker motions.

\begin{figure*}
    \centering
    \includegraphics[width=1.\linewidth]{fig_imgs/train.png}
    \caption{Training strategy. We apply distinct conditions to each of the three datasets. 
    For the HOI training, all conditions outlined in the main paper are utilized. Deviations from HOI training in Objaverse training are highlighted in red, while differences in the human training are indicated in green. 
    Missing conditions are filled to zero.}
    \label{fig:train}
\end{figure*}
\section{Training Strategy}
Due to the differences between different datasets, we propose a training strategy to integrate all dataset.
As shown in Fig.~\ref{fig:train}, we apply distinct conditions to each of the three datasets. 
For the HOI training, all conditions outlined in the main paper are utilized. Deviations from HOI training in Objaverse training are highlighted in red, while differences in the human training are indicated in green. 
None conditions are filled to zero.

\begin{figure*}
    \centering
    \includegraphics[width=1\linewidth]{fig_imgs/sup1.png}
    \caption{Qualitative comparison of different methods on HO3Dv3. Our approach achieves the best results.}
    \label{fig:sup1}
\end{figure*}

\begin{figure*}
    \centering
    \includegraphics[width=1\linewidth]{fig_imgs/sup2.png}
    \caption{Qualitative comparison of different methods on HO3Dv3. Our approach achieves the best results.}
    \label{fig:sup2}
\end{figure*}

\section{Comparisons on HO3Dv3 Dataset}
In addition to the public dataset DexYCB, we also conduct comparison on dataset HO3Dv3~\cite{ho3d}.
As shown in Figug.~\ref{fig:sup1} and Fig.~\ref{fig:sup2}, our method achieves the best results when the fingers are stacked together.
Specifically, directly learning the hand-object correspondence from 2D conditions poses an ill-posed problem, making it challenging for HOGAN to maintain consistency, particularly in scenarios where fingers are densely packed. In diffusion-based methods, the limited representation of fingers often causes details to be misinterpreted during the denoising process.

\section{More Results on Our Dataset}
In Fig.~\ref{fig:sup3} and Fig.~\ref{fig:sup4}, we show more results on our dataset.
Our method leverages the proposed multi-layer occlusion representation to effectively capture occlusion relationships based on comprehensive finger information. This approach tackles challenges such as self-occlusion of fingers, mutual occlusion between hands and objects, and the invisibility of bent fingers, leading to more accurate handling of these complex interactions.

\section{Long Sequence Generation}~\label{subsec: long}
Generating extended video sequences poses significant challenges for video diffusion models. To overcome this limitation, we adopt a temporal sliding window approach, which facilitates the generation of arbitrarily long videos while ensuring inter-frame consistency throughout.
Let $N$ denote the number of frames contained in the latent code $z$, and $w$ represent the window size with a stride of $s$. 
Therefore, $z$ will be divided into $\frac{N-w}{s} + 1$ parts.
During DDIM sampling, each timestep employs a sliding window mechanism along the temporal dimension with a specified stride to sample all groups. Overlapping segments are averaged to maintain coherence. This process is repeated across successive timesteps, ensuring consistency in sequence generation.
Formally, sampling the $p$-th window at each timestep is as follows:
\begin{align}
    \rm{DDIM}(z_{ \left[ \left(p-1\right) \times s : p \times s + s \right]} )
\end{align}
where indexes are sliced in the temporal dimension.
Temporal smoothing effectively addresses inconsistencies in overall brightness, hue, and style, which commonly arise due to noise variations and sampling discrepancies.

\section{Future Work}
In this work, driving motion sequences are extracted from our dataset.
However, our method can be integrated with motion generation methods to achieve end-to-end hand-object manipulation video generation.
For example, given the object model and motion trajectory, we first use ManiDext~\cite{zhang2024manidext} to generate motion sequences of HOI.
Then, our method leverages appearance and generated motion as inputs to produce temporally coherent and visually plausible hand-object manipulation videos, which is consistent with the main paper.

\begin{figure*}
    \centering
    \includegraphics[width=1\linewidth]{fig_imgs/sup3.png}
    \caption{Qualitative comparison of different methods on our dataset. Our approach achieves the best results.}
    \label{fig:sup3}
\end{figure*}

\begin{figure*}
    \centering
    \includegraphics[width=1\linewidth]{fig_imgs/sup4.png}
    \caption{Qualitative comparison of different methods on our dataset. Our approach achieves the best results.}
    \label{fig:sup4}
\end{figure*}
